# Supplementary material for: ProtoGS: Efficient and High-Quality Rendering with 3D Gaussian Prototypes
Source: arXiv:2503.17486 source file (2025-04-08)
Supplement: Supplementary file 1 [file X_suppl.tex]

\newpage
\clearpage
\setcounter{page}{1}
\maketitlesupplementary

\section{Overview}
Our supplementary materials contain (1) Qualitative comparison for all methods in all datasets (Fig. \ref{fig:supp_visual_results_1} and Fig. \ref{fig:supp_visual_results_2}); (2) Time comparison for all methods in all datasets (Tab. \ref{tab:training_time_comparison}); (3) Ablation analysis on the different number of initial SfM points (Tab. \ref{tab:training_time_comparison}); (4) Quantitative results of all methods on each scene across all datasets (Tab. \ref{tab:psnr_mipnerf_scores}-\ref{tab:sup_lpips_DTU}); (5) Comparison of our method with other competitors in storage size and rendering speed on every dataset (Fig. \ref{fig:sup_fps_storage_size}); (6) Comparison of our method with other competitors in visual quality and storage size on each dataset (Fig. \ref{fig:sup_quantitative_comparison}).
\begin{figure*}
    \centering
    \includegraphics{ICCV2025-Author-Kit/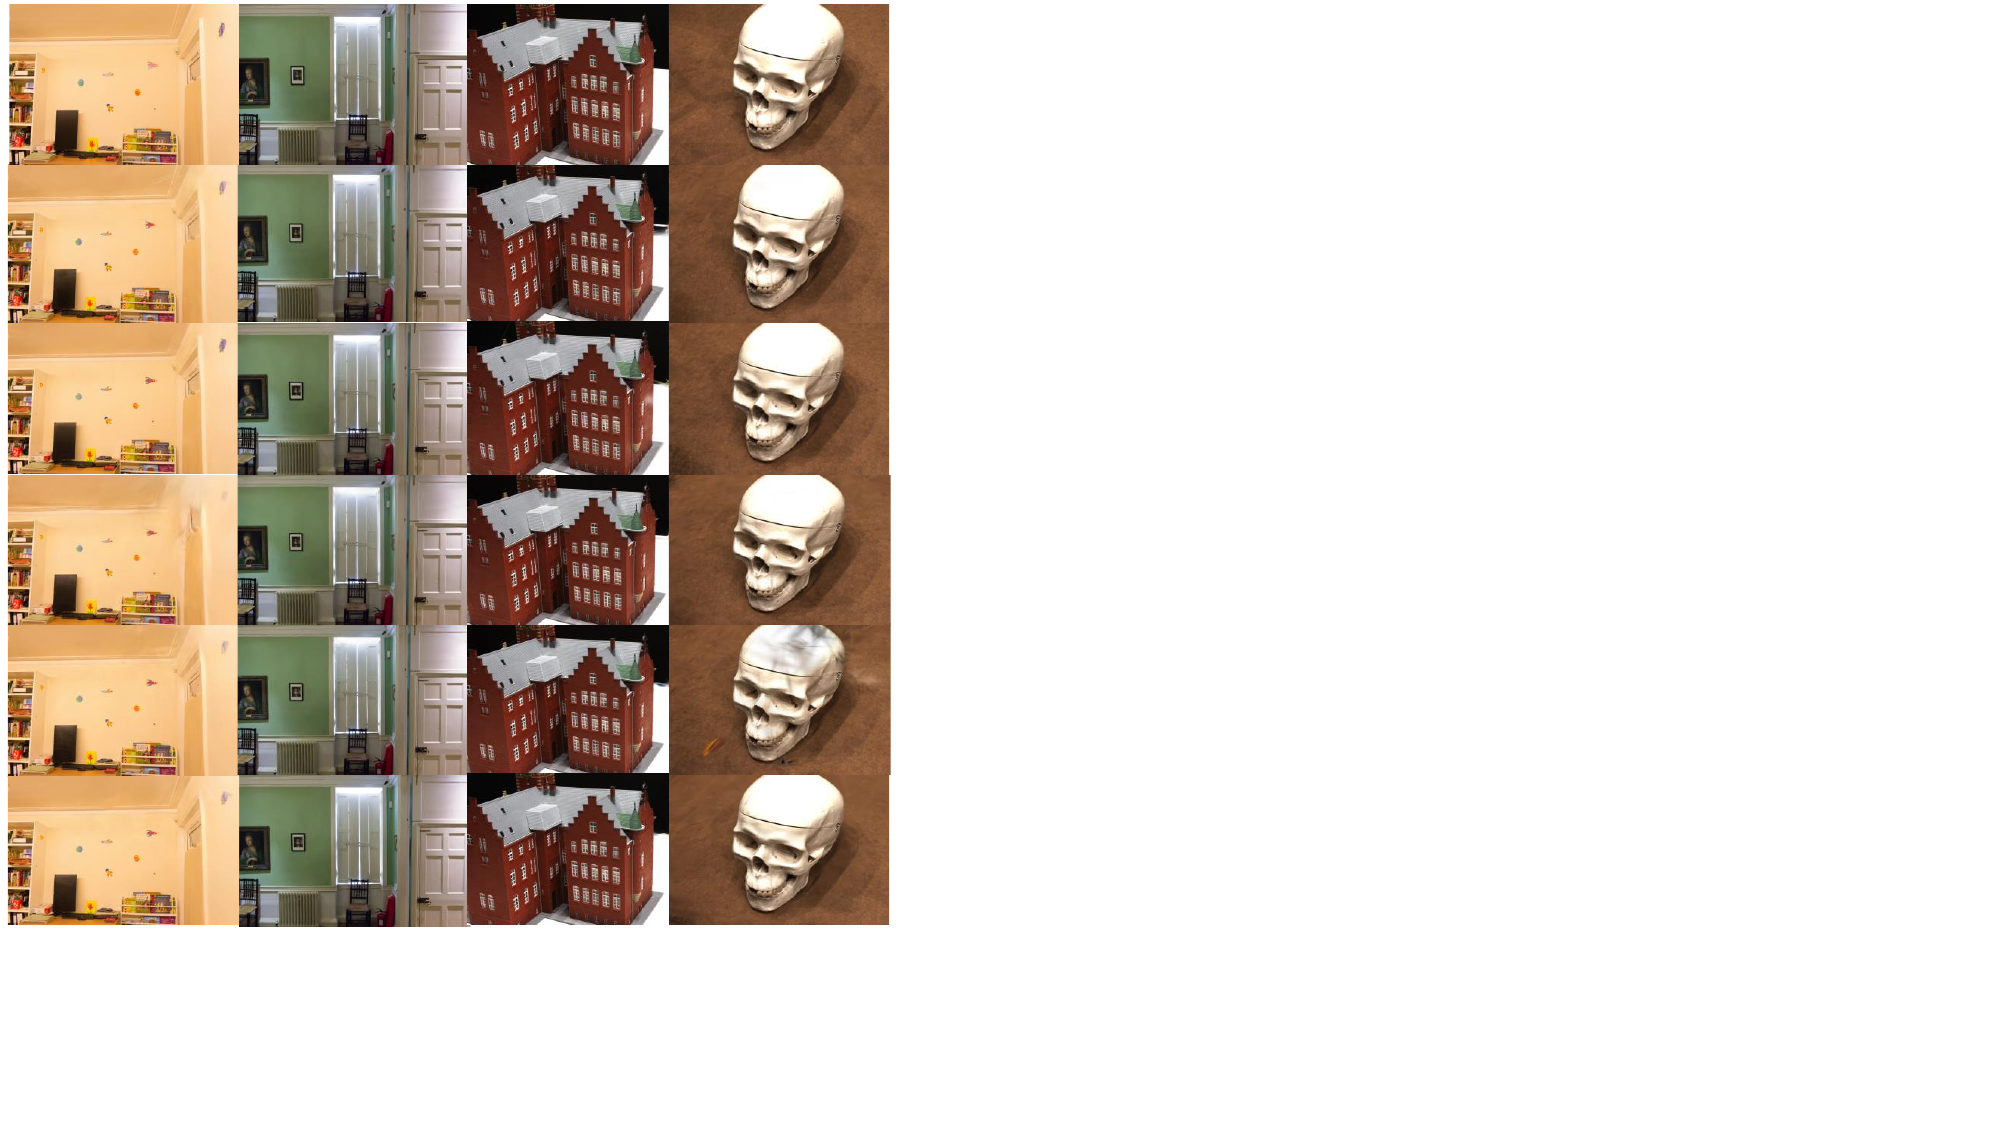}
    \caption{Extra visual results of ours and previous works. From the left column to the right, we show scenes playroom, drjohnson, DTU scan 24 and DTU scan 105. The top row shows ground-truth images. From the second row to the last rwo, we show rendered results of EAGLES, CompactGS, LightGS, 3DGS, and ProtoGS (Ours), respectively.}
    \label{fig:supp_visual_results_1}
\end{figure*}
\begin{figure*}
    \centering
    \includegraphics{ICCV2025-Author-Kit/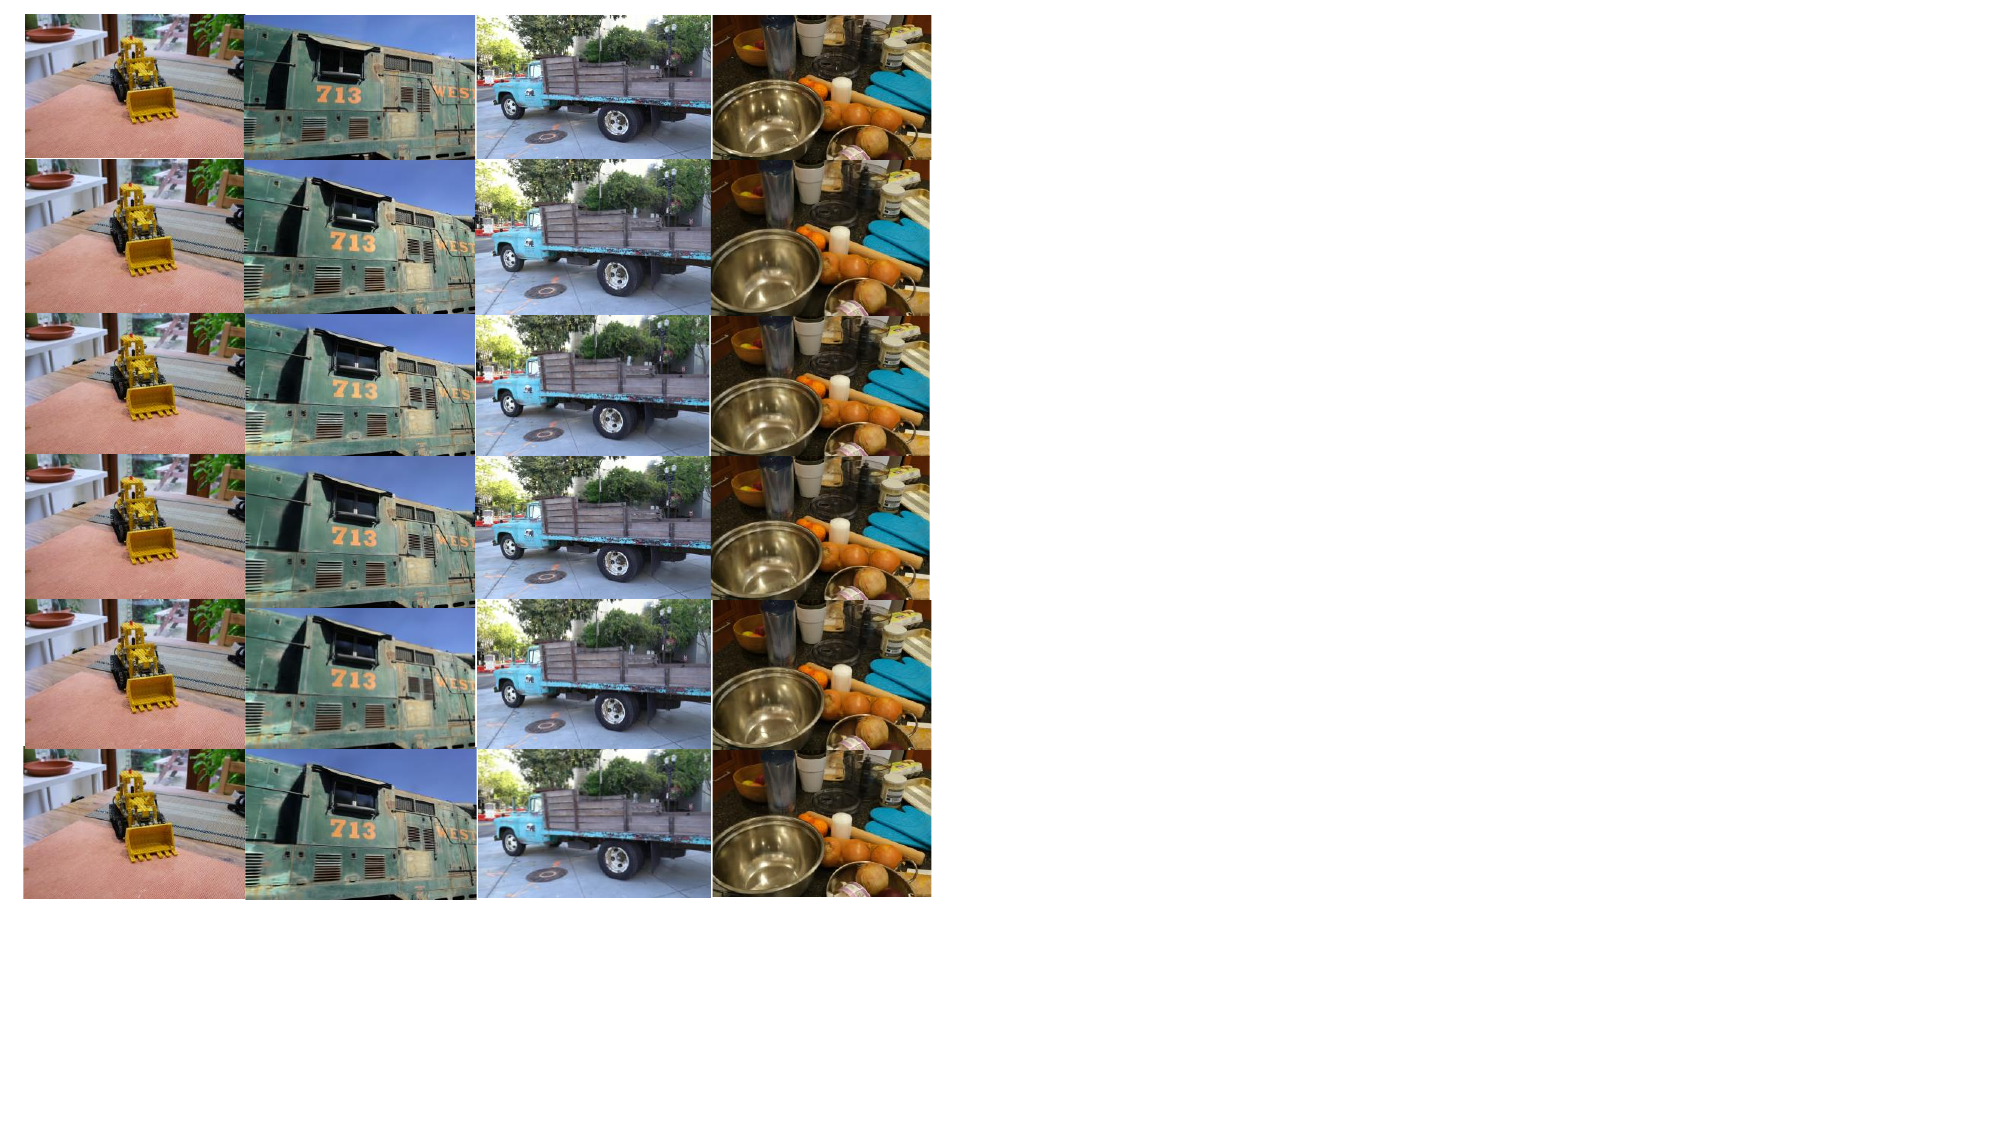}
    \caption{Extra visual results of ours and previous works. From the left column to the right, we show scenes kitchen, train, truck and counter. The top row shows grount-truth images. From the second row to the last row, we show rendered results of EAGLES, CompactGS, LightGS, 3DGS, and ProtoGS (ours), respectively.}
    \label{fig:supp_visual_results_2}
\end{figure*}
\subsection{Quantitative and qualitative results for ablation analysis}

\begin{table}[htbp]

\centering
\caption{Ablation analysis on different numbers of SfM points and time comparison with 3DGS on large-scale playroom scene.}

\begin{tabularx}{0.485\textwidth}{l|c|c|c|c|c}
\hline
\#SfM & 1/5 & 1/2 & 3/4 & 1.00 & 3DGS \\ \hline
PSNR$\uparrow$ & 30.08 & 30.02 & 30.08 & 29.98 & 30.93 \\ \hline
Time$\downarrow$ & 19.5m & 19.2m & 20.6m & 21.2m & 16.6m \\ \hline
Size$\downarrow$ & 57M & 59M & 59M & 60M & 437M \\ \hline
FPS$\uparrow$ & 272 & 270 & 270 & 270 & 105 \\ \hline
\end{tabularx}
\label{tab:training_time_comparison}
\end{table}
 We randomly sample different portions of SfM points to train our model and observe similar PSNR across different sizes, as shown in Tab. \ref{tab:training_time_comparison}, and the training time taken by different settings is slightly different. 

\begin{figure*}
    \centering
    \includegraphics[width=\linewidth]{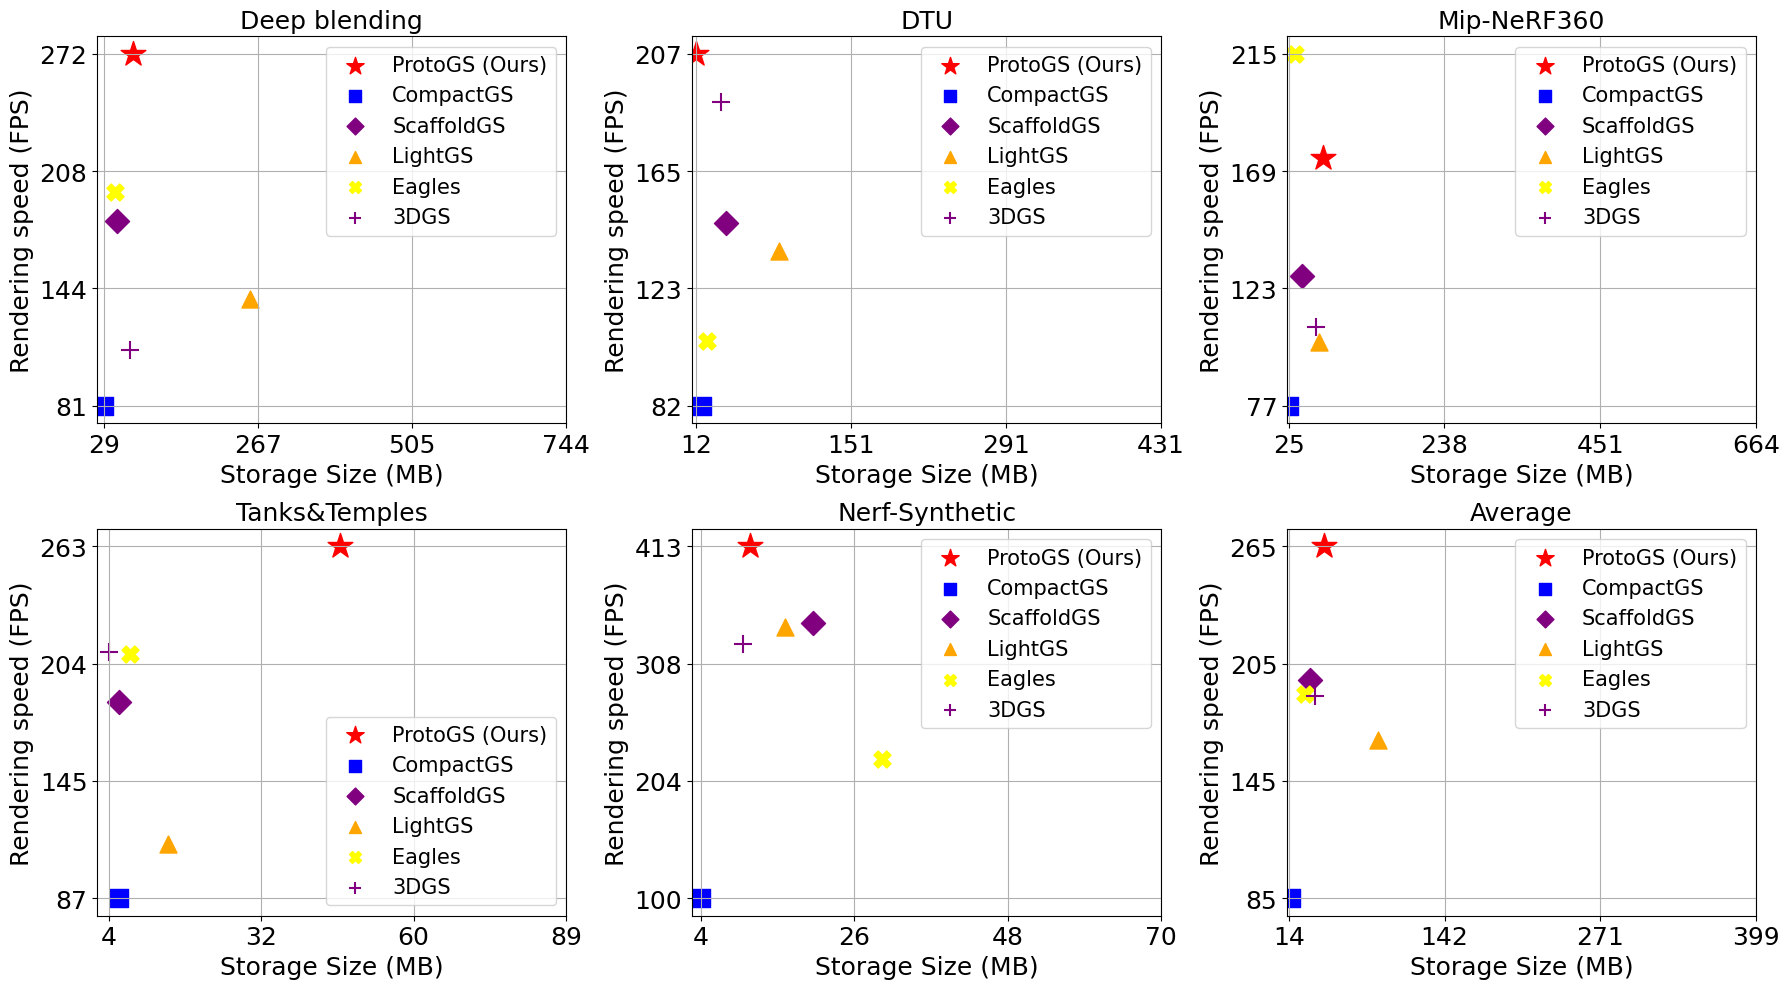}
    \caption{Comparison of our method with other competitors in storage size and rendering speed over every dataset. Our method achieves a pretty high frame rate while maintaining a low memory footprint, outperforming competitors in efficiency. The plot highlights the balance between storage requirements and rendering performance across various methods.}
    \label{fig:sup_fps_storage_size}
\end{figure*}

\begin{figure*}
    \centering
    \includegraphics[width=\linewidth]{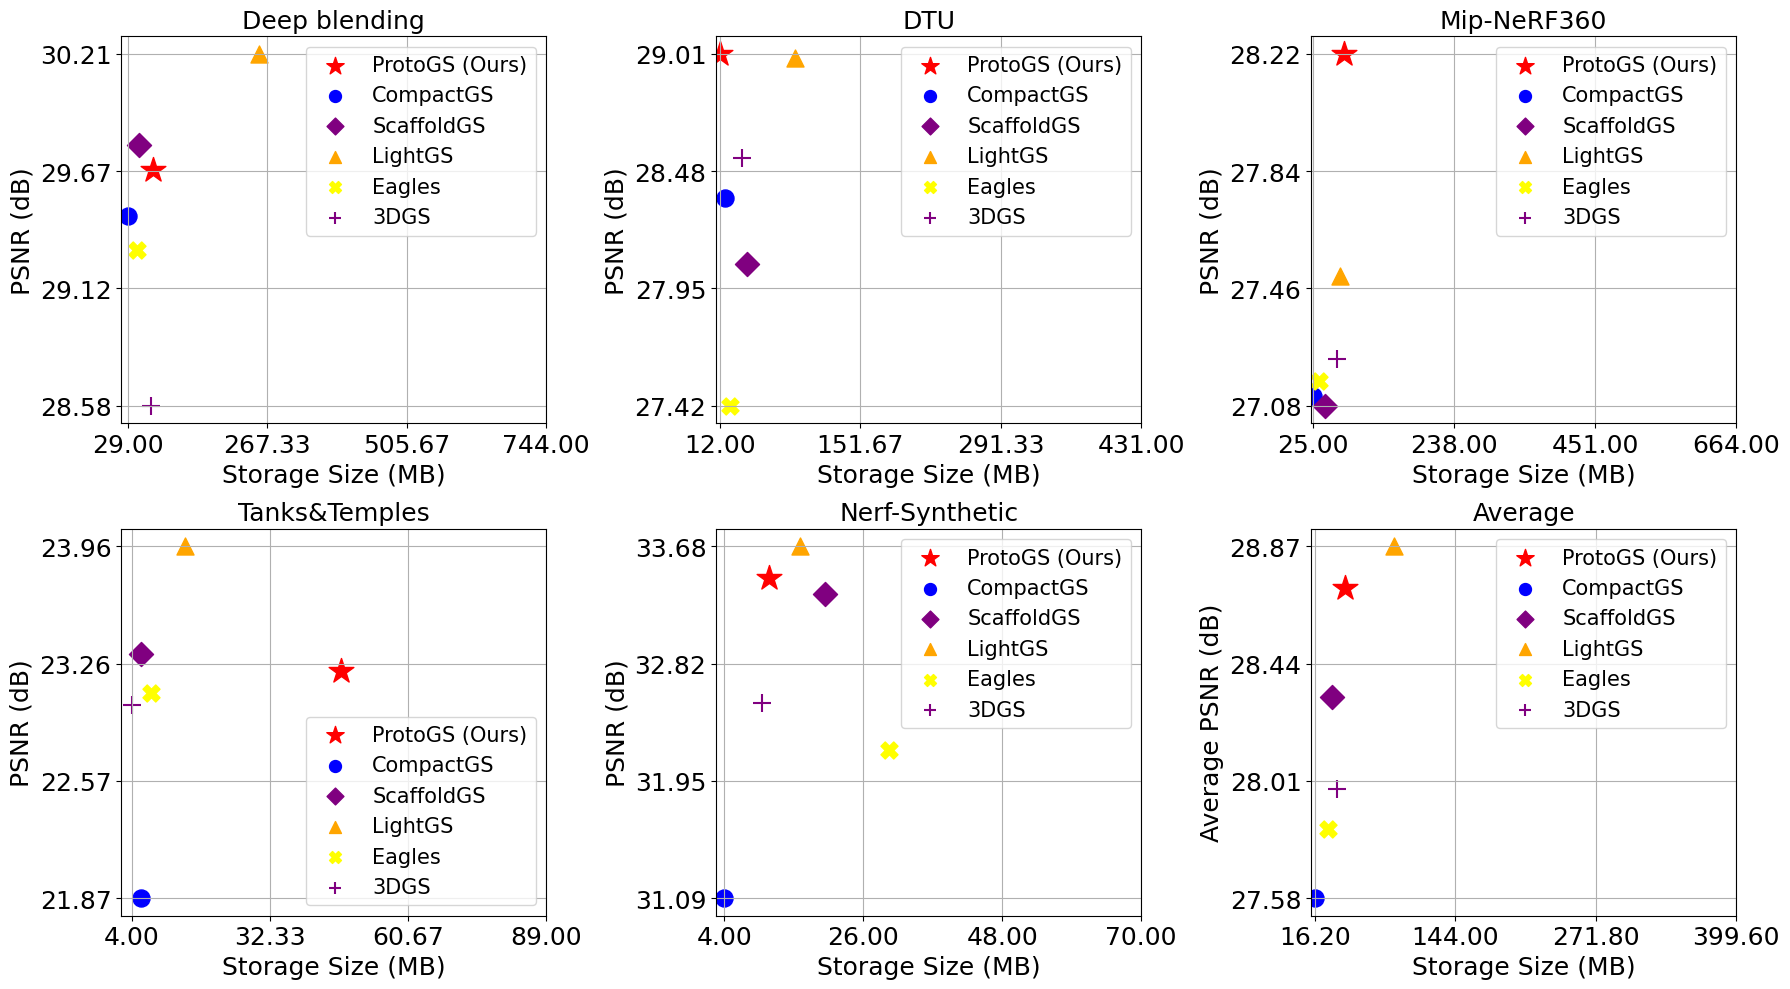}
    \caption{Comparison of our method with other competitors in visual quality and storage size over each dataset. Our method achieves high PSNR with significantly less storage, demonstrating its efficiency in maintaining quality with a reduced memory footprint. This plot highlights the balance between rendering quality and storage requirements across various methods.}
    \label{fig:sup_quantitative_comparison}
\end{figure*}
 \begin{table}
 \centering
\caption{PSNR scores for Mip-NeRF360 \cite{mipnerf360} scenes.}
 \label{tab:psnr_mipnerf_scores}
 \resizebox{\linewidth}{!}{%
 \begin{tabular}{l|ccccccc}
 \toprule
Method  & bicycle & garden & stump & room & counter & kitchen & bonsai \\
\midrule
EAGLES & 24.85& 26.69& 25.50& 29.59& 28.19& 30.41& 31.13\\
CompresGS  & 24.70& 26.68& 26.20& 31.07& 28.52& 30.62& 31.28\\
CompactGS    & 24.77& 26.81& 26.46& 30.88& 28.63& 30.47& 31.98\\
ScaffoldGS    & 24.91& 27.21& 26.38& 31.93& 29.22& 31.37& 32.42\\
LightGS   & 25.33& 26.58& 26.57& 30.51& 28.45& 30.81& 31.26\\
3DGS     & 24.88& 27.07& 26.43& 31.31& 28.87& 31.33& 32.05\\
\midrule
ProtoGS (Ours) & 24.83& 27.09& 26.27& 31.74& 28.91& 30.63& 31.63\\
\bottomrule
\end{tabular}%
}
\end{table}

\begin{table}
\centering
\caption{PSNR scores for Tanks\&Temples \cite{tanks_temple}  and Deep Blending \cite{deep_blending} scenes.}
\label{tab:psnr_scores_tanks}
\resizebox{\linewidth}{!}{
\begin{tabular}{l|cc|cc}
\toprule
Method & Truck & Train & Dr Johnson & Playroom \\
\midrule
EAGLES & 25.02& 21.17& 29.15& 29.95\\
CompresGS & 25.00& 21.59& 28.95& 29.98\\
CompactGS   & 25.02& 21.56& 29.16& 30.30\\
ScaffoldGS    & 25.78& 22.23& 29.58& 30.74\\
LightGS  & 24.74& 21.44& 26.50& 28.67\\
3DGS    & 24.60& 21.11& 30.31& 30.93\\
\midrule
ProtoGS (Ours) & 24.88& 21.55& 29.20& 30.13\\
\bottomrule
\end{tabular}
}
\end{table}

\begin{table}
\centering
\caption{PSNR scores for Synthetic Blender scenes.}
\label{tab:nerf_synthetic_psnr_scores}
\resizebox{\linewidth}{!}{
\begin{tabular}{l|cccccccc}
\midrule
Method & Mic & Chair & Ship & Materials & Lego & Drums & Ficus & Hotdog \\
\midrule
EAGLES & 35.11& 34.40& 30.57& 28.95& 34.90& 25.71& 33.64& 37.05\\
CompresGS & 35.59& 32.09& 29.49& 28.70& 33.14& 25.24& 28.81& 35.69\\
CompactGS & 35.77& 35.11& 31.26& 29.24& 35.16& 26.21& 35.25& 36.91\\
ScaffoldGS & 36.77& 35.03& 31.23& 30.60& 35.49& 26.21& 34.94& 37.72\\
LightGS & 35.43& 34.64& 30.72& 30.01& 35.48& 26.07& 35.44& 37.28\\
3DGS & 35.84& 32.34& 29.65& 28.84& 33.47& 25.34& 28.91& 36.01\\
\midrule
ProtoGS (Ours) & 35.91& 35.31& 31.21& 30.68& 35.72& 26.47& 35.24& 37.76\\
\bottomrule
\end{tabular}
}
\end{table}
\begin{table}
\centering
\caption{SSIM scores for Mip-NeRF360 \cite{mipnerf360} scenes.}
\label{tab:ssim_mipnerf_scores}
\resizebox{\linewidth}{!}{%
\begin{tabular}{l|ccccccc}
\toprule
Method  & bicycle & garden & stump & room & counter & kitchen & bonsai \\
\midrule
EAGLES  & 0.750& 0.839& 0.774& 0.926& 0.906& 0.926& 0.941\\
CompresGS  & 0.735& 0.836& 0.757& 0.921 & 0.904& 0.922 & 0.939\\
CompactGS     & 0.722& 0.831& 0.757& 0.918& 0.900& 0.919& 0.937\\
ScaffoldGS     & 0.746& 0.849& 0.765& 0.930& 0.916& 0.931& 0.948\\
LightGS    & 0.736& 0.834& 0.768& 0.915& 0.908& 0.927& 0.937\\
3DGS     & 0.747& 0.856& 0.770& 0.926& 0.915& 0.933& 0.947\\
\midrule
ProtoGS (Ours) & 0.681& 0.792& 0.778& 0.902& 0.875& 0.903& 0.902\\
\bottomrule
\end{tabular}
}
\end{table}
\begin{table}
\centering
\caption{SSIM scores for Synthetic Blender \cite{NeRF_field} scenes.}
\label{tab:nerf_synthetic_ssim_scores}
\resizebox{\linewidth}{!}{
\begin{tabular}{l|cccccccc}
\midrule
Method & Mic & Chair & Ship & Materials & Lego & Drums & Ficus & Hotdog \\
\midrule
EAGLES   & 0.989& 0.984& 0.896& 0.949& 0.980& 0.950& 0.982& 0.983\\
CompresGS & 0.989 & 0.982 & 0.890 & 0.952& 0.975& 0.942& 0.957& 0.981\\
CompactGS    & 0.991& 0.983 & 0.985& 0.954& 0.979& 0.951& 0.987& 0.983\\
ScaffoldGS     & 0.992& 0.985& 0.901& 0.960& 0.980& 0.947& 0.984& 0.983\\
LightGS   & 0.991& 0.987& 0.899& 0.959& 0.981& 0.954& 0.987& 0.983\\
3DGS & 0.989& 0.984& 0.891& 0.953& 0.978& 0.944& 0.959& 0.982\\
\midrule
ProtoGS (Ours) & 0.985 & 0.980 & 0.899 & 0.953 & 0.974 & 0.951 & 0.985 & 0.986 \\
\bottomrule
\end{tabular}
}
\end{table}

\begin{table}
\centering
\caption{SSIM scores for Tanks\&Temples \cite{tanks_temple} and Deep Blending \cite{deep_blending} scenes.}
\label{tab:ssim_scores_tanks}
\resizebox{\linewidth}{!}{
\begin{tabular}{l|cc|cc}
\toprule
Method & Truck & Train & Dr Johnson & Playroom \\
\midrule
EAGLES   & 0.872& 0.794& 0.901& 0.907\\
CompresGS  & 0.872& 0.803& 0.897& 0.901\\
CompactGS    & 0.870& 0.792& 0.899& 0.900\\
ScaffoldGS     & 0.882& 0.820& 0.903& 0.907\\
LightGS   & 0.863& 0.777& 0.866& 0.884\\
3DGS    & 0.882& 0.813& 0.900& 0.907\\
\midrule
ProtoGS (Ours) & 0.857& 0.760& 0.896& 0.906\\
\bottomrule
\end{tabular}
}
\end{table}

\begin{table}
\centering
                                                                                                                                                                                                        \caption{LPIPS scores for Mip-NeRF360 \cite{mipnerf360} scenes.}
                                                                                                                                                                                                        \label{tab:lpips_mipnerf_scores}
                                                                                                                                                                                                        \resizebox{\linewidth}{!}{%
                                                                                                                                                                                                        \begin{tabular}{l|ccccccc}
                                                                                                                                                                                                        \toprule
                                                                                                                                                                                                        Method  & bicycle & garden & stump & room & counter & kitchen & bonsai \\
                                                                                                                                                                                                        \midrule
                                                                                                                                                                                                        EAGLES    & 0.245& 0.155& 0.242& 0.201& 0.199& 0.128& 0.193\\
                                                                                                                                                                                                        CompresGS  & 0.269& 0.157
& 0.273& 0.212& 0.199& 0.131& 0.195\\
                                                                                                                                                                                                        CompactGS     & 0.287& 0.161& 0.280& 0.209& 0.206& 0.130& 0.193\\
                                                                                                                                                                                                        ScaffoldGS     & 0.257& 0.135& 0.260& 0.187& 0.185& 0.118& 0.180\\
                                                                                                                                                                                                        LightGS    & 0.270& 0.152& 0.259& 0.226& 0.208& 0.134& 0.203\\
                                                                                                                                                                                                        3DGS     & 0.244& 0.122& 0.241& 0.197& 0.184& 0.116& 0.180\\
                                                                                                                                                                                                        \midrule
                                                                                                                                                                                                        ProtoGS (Ours) & 0.250& 0.151& 0.227& 0.178& 0.196& 0.134& 0.195\\
                                                                                                                                                                                                        \bottomrule
                                                                                                                                                                                                        \end{tabular}%
                                                                                                                                                                                                        }
                                                                                                                                                                                                        \end{table}
                                                                                                                                                                                                        
                                                                                                                                                                                                        \begin{table}
                                                                                                                                                                                                        \centering
                                                                                                                                                                                                        \caption{LPIPS scores for Tanks\&Temples \cite{tanks_temple} and Deep Blending \cite{deep_blending} scenes.}
                                                                                                                                                                                                        \label{tab:lpips_scores_tanks}
                                                                                                                                                                                                        \resizebox{\linewidth}{!}{
                                                                                                                                                                                                        \begin{tabular}{l|cc|cc}
                                                                                                                                                                                                        \toprule
                                                                                                                                                                                                        Method & Truck & Train & Dr Johnson & Playroom \\
                                                                                                                                                                                                        \midrule
                                                                                                                                                                                                        EAGLES   & 0.165& 0.242& 0.244& 0.254\\
                                                                                                                                                                                                        CompresGS & 0.159& 0.222& 0.258& 0.260\\
                                                                                                                                                                                        CompactGS    & 0.163& 0.240& 0.258& 0.259\\
                                                                                                                                                                                                        ScaffoldGS     & 0.143& 0.206& 0.256& 0.255\\
                                                                                                                                                                                                        LightGS   & 0.176& 0.276& 0.310& 0.293\\
                                                                                                                                                                                                        3DGS    & 0.147& 0.207& 0.244& 0.244\\
                                                                                                                                                                                                        \midrule
                                                                                                                                                                                                        ProtoGS (Ours) & 0.150& 0.206& 0.268& 0.263\\
                                                                                                                                                                                                        \bottomrule
                                                                                                                                                                                                        \end{tabular}
                                                                                                                                                                                                        }
                                                                                                                                                                                                        \end{table}
                                                                                                                                                                                                        
                                                                                                                                                                                                        \begin{table}
                                                                                                                                                                                                        \centering
                                                                                                                                                                                                        \caption{LPIPS scores for Synthetic Blender \cite{NeRF_field} scenes.}
                                                                                                                                                                                                        \label{tab:nerf_synthetic_lpips_scores}
                                                                                                                                                                                                        \resizebox{\linewidth}{!}{
                                                                                                                                                                                                        \begin{tabular}{l|cccccccc}
                                                                                                                                                                                                        \midrule
                                                                                                                                                                                                        Method & Mic & Chair & Ship & Materials & Lego & Drums & Ficus & Hotdog \\
                                                                                                                                                                                                        \midrule
                                                                                                                                                                                                        EAGLES   & 0.011& 0.015& 0.127& 0.054& 0.021& 0.045& 0.018& 0.025\\
                                                                                                                                                                                                        CompresGS & 0.025& 0.023& 0.063& 0.065& 0.033& 0.063& 0.039& 0.037\\
                                                                                                                                                                                                        CompactGS    & 0.008& 0.013& 0.115& 0.020& 0.020& 0.042& 0.013& 0.023\\
                                                                                                                                                                                                        ScaffoldGS     & 0.007& 0.013& 0.109& 0.041& 0.019& 0.048& 0.014& 0.023\\
                                                                                                                                                                                                        LightGS   & 0.009& 0.014& 0.121& 0.043& 0.021& 0.042& 0.013& 0.034\\
                                                                                                                                                                                                        3DGS & 0.043& 0.024& 0.140& 0.137& 0.067& 0.065& 0.059& 0.036\\
                                                                                                                                                                                                        \midrule
                                                                                                                                                                                                        ProtoGS (Ours) & 0.034 & 0.027 & 0.018 & 0.066 & 0.068 & 0.042 & 0.022 & 0.071 \\
                                                                                                                                                                                                        \bottomrule
                                                                                                                                                                                                        \end{tabular}
                                                                                                                                                                                                        }
                                                                                                                                                                                                        \end{table}

                                                                                                                                                                                                        \begin{table*}[!t]
                                                                                                                                                                                                        \centering
                                                                                                                                                                                                        \caption{PSNR scores for DTU scenes.}
                                                                                                                                                                                                        \label{tab:sup_psnr_DTU}
                                                                                                                                                                                                        \setlength{\tabcolsep}{1.55pt} % Adjust the column spacing
                                                                                                                                                                                                        \begin{tabularx}{\linewidth}{lccccccccccccc}
                                                                                                                                                                                                        \toprule
                                                                                                                                                                                                        Method & scan24 & scan37 & scan40 & scan55 & scan63 & scan65 & scan69 & scan83 & scan97 & scan105 & scan106 & scan110 & scan114 \\
                                                                                                                                                                                                        \midrule
                                                                                                                                                                                                        EAGLES & 27.06 & 25.16 & 26.11 & 27.92 & 31.48 & 28.21 & 27.10 & 28.21 & 24.93 & 26.88 & 32.53 & 30.45 & 28.48 \\
                                                                                                                                                                                                        CompresGS & 26.57 & 25.40 & 25.92 & 28.33 & 31.12 & 29.28 & 26.50 & 26.77 & 24.92 & 26.88 & 32.53 & 30.15 & 27.98 \\
                                                                                                                                                                                                        CompactGS & 25.63 & 23.40 & 25.22 & 27.88 & 30.80 & 28.99 & 25.69 & 27.32 & 24.74 & 26.09 & 30.98 & 29.40 & 28.19  \\
                                                                                                                                                                                                        ScaffoldGS & 23.67 & 25.50 & 25.45 & 30.47 & 26.81 & 26.84 & 28.77 & 32.93 & 30.47 & 29.33 & 33.65 & 33.05 & 29.13 \\
                                                                                                                                                                                                        LightGS & 25.29 & 24.75 & 24.46 & 27.66 & 30.34 & 28.73 & 26.63 & 22.56 & 22.60 & 26.50 & 32.17 & 30.40 & 26.42  \\
                                                                                                                                                                                                        3DGS & 26.66 & 25.46& 25.80 & 28.53 & 31.31 & 29.18 & 26.62 & 26.80 & 24.49 & 27.31 & 32.10 & 30.43 & 28.06 \\
                                                                                                                                                                                                        \midrule
                                                                                                                                                                                                        ProtoGS (Ours) & 27.20 & 25.25 & 25.80 & 27.72 & 20.84 & 28.96 & 26.94 & 27.22 & 25.99 & 27.78 & 31.92 & 29.70 & 28.50  \\
                                                                                                                                                                                                        \bottomrule
                                                                                                                                                                                                        \end{tabularx}
                                                                                                                                                                                                        \end{table*}

                                                                                                                                                                                                        \begin{table*}[!t]
                                                                                                                                                                                                        \centering
                                                                                                                                                                                                        \caption{SSIM scores for DTU  scenes.}
                                                                                                                                                                                                        \label{tab:sup_ssim_DTU}
                                                                                                                                                                                                        \setlength{\tabcolsep}{1.55pt} % Adjust the column spacing
                                                                                                                                                                                                        \begin{tabularx}{\linewidth}{lccccccccccccc}
                                                                                                                                                                                                        \toprule
                                                                                                                                                                                                        Method & scan24 & scan37 & scan40 & scan55 & scan63 & scan65 & scan69 & scan83 & scan97 & scan105 & scan106 & scan110 & scan114 \\
                                                                                                                                                                                                        \midrule
                                                                                                                                                                                                        EAGLES & 0.914 & 0.901 & 0.901 & 0.900 & 0.874 & 0.945 & 0.872 & 0.873 & 0.862 & 0.845 & 0.908 & 0.888 & 0.882 \\
                                                                                                                                                                                                        CompresGS & 0.912 & 0.896 & 0.887 & 0.862 & 0.944 & 0.865 & 0.865 & 0.856 & 0.838 & 0.869 & 0.903 & 0.887 & 0.871 \\
                                                                                                                                                                                                        CompactGS  & 0.902 & 0.878 & 0.876 & 0.854 & 0.935 & 0.861 & 0.846 & 0.850 & 0.835 & 0.857 & 0.893 & 0.869 & 0.870  \\
                                                                                                                                                                                                        ScaffoldGS & 0.890 & 0.890 & 0.878 & 0.940 & 0.857 & 0.859 & 0.870 & 0.906 & 0.882 & 0.880 & 0.900 & 0.898 & 0.865 \\
                                                                                                                                                                                                        LightGS& 0.910 & 0.894 & 0.887 & 0.852 & 0.941 & 0.855 & 0.857 & 0.815 & 0.813 & 0.860 & 0.901 & 0.881 & 0.859  \\
                                                                                                                                                                                                        3DGS  & 0.912 & 0.899 & 0.888 & 0.863 & 0.944 & 0.864 & 0.864 & 0.854 & 0.838 & 0.868 & 0.902 & 0.888 & 0.870 \\
                                                                                                                                                                                                        \midrule
                                                                                                                                                                                                        ProtoGS (Ours) & 0.901 & 0.890 & 0.870 & 0.830 & 0.929 & 0.840 & 0.847 & 0.840 & 0.848 & 0.850 & 0.890 & 0.880 & 0.867  \\
                                                                                                                                                                                                        \bottomrule
                                                                                                                                                                                                        \end{tabularx}
                                                                                                                                                                                                        \end{table*}
                                                                                                                                                                                                        
                                                                                                                                                                                                        \begin{table*}[!t]
                                                                                                                                                                                                        \centering
                                                                                                                                                                                                        \caption{LPIPS scores for DTU  scenes.}
                                                                                                                                                                                                        \label{tab:sup_lpips_DTU}
                                                                                                                                                                                                        \setlength{\tabcolsep}{1.55pt} % Adjust the column spacing
                                                                                                                                                                                                        \begin{tabularx}{\linewidth}{lccccccccccccc}
                                                                                                                                                                                                        \toprule
                                                                                                                                                                                                        Method & scan24 & scan37 & scan40 & scan55 & scan63 & scan65 & scan69 & scan83 & scan97 & scan105 & scan106 & scan110 & scan114 \\
                                                                                                                                                                                                        \midrule
                                                                                                                                                                                                        EAGLES  & 0.136 & 0.198 & 0.192 & 0.269 & 0.166 & 0.315 & 0.298 & 0.372 & 0.338 & 0.329 & 0.321 & 0.360 & 0.319 \\
                                                                                                                                                                                                        CompresGS  & 0.138 & 0.204 & 0.210 & 0.305 & 0.171 & 0.331 & 0.310 & 0.384 & 0.348 & 0.336 & 0.332 & 0.365 & 0.327 \\
                                                                                                                                                                                                        CompactGS  & 0.148 & 0.215 & 0.220 & 0.312 & 0.187 & 0.346 & 0.338 & 0.395 & 0.356 & 0.356 & 0.341 & 0.391 & 0.334  \\
                                                                                                                                                                                                        ScaffoldGS & 0.165 & 0.222 & 0.237 & 0.179 & 0.345 & 0.336 & 0.337 & 0.333 & 0.384 & 0.334 & 0.347 & 0.350 & 0.314 \\
                                                                                                                                                                                                        LightGS& 0.147 & 0.210 & 0.208 & 0.314 & 0.184 & 0.354 & 0.332 & 0.423 & 0.376 & 0.358 & 0.338 & 0.375 & 0.346  \\
                                                                                                                                                                                                        3DGS & 0.133 & 0.195 & 0.197 & 0.298 & 0.167 & 0.326 & 0.304 & 0.380 & 0.342 & 0.331 & 0.327 & 0.359 & 0.321 \\
                                                                                                                                                                                                        \midrule
ProtoGS (Ours) & 0.171 & 0.230 & 0.250 & 0.370 & 0.208 & 0.386 & 0.369 & 0.430 & 0.361 & 0.390 & 0.370 & 0.369 & 0.361  \\
                                                                                                                                                                                                        \bottomrule
                                                                                                                                                                                                        \end{tabularx}
                                                                                                                                                                                                        \end{table*}
\begin{table*}[htbp]

\centering
\caption{Ablation analysis on different datasets and time comparison across all methods.}

\begin{tabularx}{0.725\textwidth}{l|c|c|c|c|c}
\hline
Dataset & DB & DTU & M-NeRF360 & T\&T & NeRF-Synthetic \\ 
\midrule
EAGLES & 30m24s & 48m53s & 21m34s & 11m39s & 15m34s \\ 
EAGLES & 30m24s & 48m53s & 21m34s & 11m39s & 15m34s \\ 
CompactGS & 23m59s & 31m35s & 43m09s & 15m56s & 8m04s \\
ScaffoldGS & 21m47s & 20m46s & 26m15ss & 17m59s & 20m40s \\
LightGS & 21m03s & 21m05s & 23m47s & 21m03s & 15m32s \\ 
3DGS & 21m52s & 31m31s & 24m07s & 13m51s & 6m11s \\
ProtoGS (Ours) & 31m03s & 27m54s & 49m35s & 46m16s & 6m08s \\
\bottomrule
\end{tabularx}
\label{tab:training_time_comparison_all_data}
\end{table*}
